# Supplementary material for: On Multi-Relational Link Prediction with Bilinear Models
Source: arXiv:1709.04808 source file (2017-09-14)
Supplement: Supplementary file 1 [file 8-appendix.tex]

% !TEX root = main.tex
\newpage
\section{Online Appendix}

\subsection{Details for Proof of Th.~\ref{thm:R_from_T}} 
Define $\va_i$, $\mR_k$, $\va_i'$, and $\mR_k'$ as in the proof of Th.~\ref{thm:R_from_T}. Observe that
\begin{align*}
  (\va_i')^T \underbrace{\begin{pmatrix}
      \vzero_{r\times r} & \vzero_{r\times r} & 0 \\
      \vzero_{r\times r} & \vzero_{r\times r} & 0 \\
      \ve_{1,r}^T & \vzero_{1\times r} & 0
    \end{pmatrix}}_{\mR_k^{11}} \va_j' &= (\va_i')^T \begin{pmatrix}
    \vzero_r \\
    \vzero_r \\
    1
  \end{pmatrix} = \va_i^T\va_i \allowdisplaybreaks[1] \\
      %%%
  (\va_i')^T \underbrace{\begin{pmatrix}
      \vzero_{r\times r} & \vzero_{r\times r} & 1 \\
      \vzero_{r\times r} & \vzero_{r\times r} & 0 \\
      \vzero_{1\times r}^T & \vzero_{1\times r} & 0
    \end{pmatrix}}_{\mR_k^{22}} \va_j' &= (\va_i')^T \begin{pmatrix}
    \va_j^T\va_j\\
    \vzero_r \\
    \vzero_r
  \end{pmatrix} = \va_j^T\va_j \allowdisplaybreaks[1] \\
      %%%
  (\va_i')^T \underbrace{\begin{pmatrix}
      \vzero_{r\times r} & \vzero_{r\times r} & 0\\
      \vzero_{r\times r} & \mI_{r\times r} & 0 \\
      \vzero_{1\times r} & \vzero_{1\times r} & 0
    \end{pmatrix}}_{\mR_{k}^{12}} \va_j' &= (\va_i')^T
                                           \begin{pmatrix}
                                             \vzero_r \\ \va_j \\ 0
                                           \end{pmatrix}
  = \va_i^T\va_j \allowdisplaybreaks[1] \\
      %%%
  (\va_i')^T \underbrace{\begin{pmatrix}
      \vzero_{r\times r} & \vzero_{r\times r} & 0\\
      \diag{\vr_k} & \vzero_{r\times r} & 0 \\
      \vzero_{1\times r} & \vzero_{1\times r} & 0
    \end{pmatrix}}_{\mR_{k}^{13}} \va_j' &= (\va_i')^T
                                           \begin{pmatrix}
                                             \vzero_r \\ \vr_k \\ 0
                                           \end{pmatrix}
  = \va_i^T\vr_k \allowdisplaybreaks[1] \\
      %%%
  (\va_i')^T \underbrace{\begin{pmatrix}
      \vzero_{r\times r} & \diag{\vr_k} & 0\\
      \vzero_{r\times r} & \vzero_{r\times r} & 0 \\
      \vzero_{1\times r} & \vzero_{1\times r} & 0
    \end{pmatrix}}_{\mR_{k}^{23}} \va_j' &=
                                           \begin{pmatrix}
                                             \vzero_r^T & \vr_k^T & 0
                                           \end{pmatrix} \va_j' = \va_j^T\vr_k
\end{align*}
 
Using these observations, we obtain
\begin{align*}
  s_k^\text{m}(i,j) &= -\norm{\va_i+\vr_k - \va_j}^2_2 \allowdisplaybreaks[1] \\
                    &= -\langle \va_i+\vr_k - \va_j, \va_i+\vr_k - \va_j \rangle \allowdisplaybreaks[1] \\
                    &= -(\va_i^T(\va_i+\vr_k - \va_j) + \vr_k^T(\va_i+\vr_k - \va_j) \\ 
                    & \quad -\va_j^T(\va_i+\vr_k - \va_j)) \allowdisplaybreaks[1] \\
                    &= -(\va_i^T\va_i+\va_j^T\va_j+2\va_i^T\vr_k - 2\va_i^T\va_j \\
                    & \quad -2\va_j^T\vr_k + \vr_k^T\vr_k) \allowdisplaybreaks[1] \\
                    &= -((\va_i')^T(\underbrace{\mR_k^{11}+\mR_k^{22}+2\mR_k^{13}-2\mR_k^{12}-2\mR_k^{23}}_{-\mR_k'})\va_j' \\
                    & \quad  + \vr_k^T\vr_k) \allowdisplaybreaks[1] \\
                    &= (\va_i')^T\mR_k'\va_j' - c_k
\end{align*}
where $c_k=\vr_k^T\vr_k$ is a relation-dependent constant. Now,
\begin{align*}
  &s_k^{m_R}(i,j) \le s_k^{m_R}(i',j') \\
  \iff &(\va_i')^T\mR_k'\va_j' \le (\va_{i'}')^T\mR_k'\va_{j'}' \\
  \iff &s_k^{m_T}(i,j) \le s_k^{m_T}(i',j').
\end{align*}
